# Supplementary material for: An Analysis of Logit Learning with the r-Lambert Function
Source: arXiv:2409.05044 source file (2025-02-16)
Supplement: Supplementary file 1 [file appendix.tex]

% !TEX root = main.tex

%%%% Subsection %%%%
\subsection{Proof of Lemma \ref{lma:h0h1sps}}\label{ap:h0h1sps}
\input{./Proofs/Lemmas/Prf-Lma-h0h1sps}

%%%% Subsection %%%%
\subsection{Proof of Lemma \ref{lma:h0h1sps}}\label{ap:h0h1rts}
\input{./Proofs/Lemmas/Prf-Lma-h0h1rts}

%%%% Subsection %%%%
\subsection{Proof of Theorem \ref{thm:AsympOfFPs}}\label{ap:asympFP}
\input{./Proofs/"Asymptotics of Fixed Points"/Prf-orgFpLimits}

\input{./Proofs/"Asymptotics of Fixed Points"/Prf-q1FpLimits}

\input{./Proofs/"Asymptotics of Fixed Points"/Prf-q2FpLimits}

\input{./Proofs/"Asymptotics of Fixed Points"/Prf-q3FpLimits}

\input{./Proofs/"Asymptotics of Fixed Points"/Prf-q4FpLimits}

%%%% Subsection %%%%
\subsection{Proof of Theorem \ref{thm:AsympFPStab}}\label{ap:AsympFPStab}
\input{./Proofs/"Stability of Fixed Points"/Prf-AsympFPStab2}
